# Supplementary material for: Step Growth and Meandering in a Precursor-Mediated Epitaxy with Anisotropic Attachment Kinetics and Terrace Diffusion
Source: arXiv:1403.6812 source file (2015-06-16)
Supplement: Supplementary file 1 [file supplement.pdf]

**Coefficients of Eq. (25) :**

$$
\begin{aligned}
p_{1\,(2)} = {} & -\Bigg(d_{11}\,q_1 + \frac{d_{11}\,q_2\,(\alpha_1-\alpha_3)\,(-1+d_{22}\,\alpha_1\,\beta_0\,(1+\Upsilon_{k,m}))}{\alpha_1+\alpha_3} - \Big(\Big(\hat{\chi}\,d_{11}\,\alpha_2\,\big(d_{22}\,(2\,\alpha_1+\alpha_3)+\hat{\beta}_a\big) + 2\,d_0 \\
& \quad d_{22}^2\,\alpha_3\,(\alpha_1+\alpha_3)^2\,\big(d_{22}\,\alpha_1+\hat{\beta}_a\big)\,(1+\epsilon_{s,m})\Big)\,(1+d_{22}\,\alpha_3\,\beta_0\,(1+\Upsilon_{k,m}))\Big)\Big/ \\
& \quad \Big(d_{22}\,(\alpha_1+\alpha_3)^2\,\big(d_{22}\,\alpha_1+\hat{\beta}_a\big)\Big)\Bigg)\Big/\Big(2\,(1+d_{22}\,\alpha_3\,\beta_0\,(1+\Upsilon_{k,m}))^2\Big)
\end{aligned}
$$

---

$$
\begin{aligned}
p_{1\,(4)} = {} & \frac{1}{8\,d_{22}^2\,(1+d_{22}\,\alpha_3\,\beta_0\,(1+\Upsilon_{k,m}))^3}\,\beta_0\,(1+\Upsilon_{k,m}) \\
& \Big((d_{12}+d_{21})\,d_{22}\,q_1\,(d_{12}\,(-1+5\,d_{22}\,\alpha_3\,\beta_0\,(1+\Upsilon_{k,m})) - d_{21}\,(1+7\,d_{22}\,\alpha_3\,\beta_0\,(1+\Upsilon_{k,m}))) + \\
& \quad 1\Big/(\alpha_1+\alpha_3)^2\,d_{22}\,q_2\,\Big((d_{12}+d_{21})\,\alpha_3^2 \\
& \qquad (d_{12}\,(-1+5\,d_{22}\,\alpha_3\,\beta_0\,(1+\Upsilon_{k,m})) - d_{21}\,(1+7\,d_{22}\,\alpha_3\,\beta_0\,(1+\Upsilon_{k,m}))) + (d_{12}+d_{21})\,d_{22} \\
& \qquad \alpha_1^3\,\beta_0\,(1+\Upsilon_{k,m})\,(d_{12}\,(-1+5\,d_{22}\,\alpha_3\,\beta_0\,(1+\Upsilon_{k,m})) - d_{21}\,(1+7\,d_{22}\,\alpha_3\,\beta_0\,(1+\Upsilon_{k,m}))) + \\
& \qquad \alpha_1\,\alpha_3\,\Big(-2\,d_{12}\,d_{21}\,\big(2+3\,d_{22}\,\alpha_3\,\beta_0\,(1+\Upsilon_{k,m}) + d_{22}^2\,\alpha_3^2\,\beta_0^2\,(1+\Upsilon_{k,m})^2\big) + \\
& \qquad\quad d_{12}^2\,\big(-2+5\,d_{22}\,\alpha_3\,\beta_0\,(1+\Upsilon_{k,m}) + d_{22}^2\,\alpha_3^2\,\beta_0^2\,(1+\Upsilon_{k,m})^2\big) - \\
& \qquad\quad d_{21}^2\,\big(2+11\,d_{22}\,\alpha_3\,\beta_0\,(1+\Upsilon_{k,m}) + 3\,d_{22}^2\,\alpha_3^2\,\beta_0^2\,(1+\Upsilon_{k,m})^2\big)\Big) + \\
& \qquad \alpha_1^2\,\Big(d_{12}^2\,\big(-5-9\,d_{22}\,\alpha_3\,\beta_0\,(1+\Upsilon_{k,m}) + 2\,d_{22}^2\,\alpha_3^2\,\beta_0^2\,(1+\Upsilon_{k,m})^2\big) - \\
& \qquad\quad 2\,d_{12}\,d_{21}\,\big(5+11\,d_{22}\,\alpha_3\,\beta_0\,(1+\Upsilon_{k,m}) + 6\,d_{22}^2\,\alpha_3^2\,\beta_0^2\,(1+\Upsilon_{k,m})^2\big) - \\
& \qquad\quad d_{21}^2\,\big(5+13\,d_{22}\,\alpha_3\,\beta_0\,(1+\Upsilon_{k,m}) + 14\,d_{22}^2\,\alpha_3^2\,\beta_0^2\,(1+\Upsilon_{k,m})^2\big)\Big)\Big) - \\
& \quad 1\Big/\Big((\alpha_1+\alpha_3)^3\,\big(d_{22}\,\alpha_1+\hat{\beta}_a\big)^2\Big)\,\hat{\chi}\,(d_{12}+d_{21})\,\alpha_2\,(1+d_{22}\,\alpha_3\,\beta_0\,(1+\Upsilon_{k,m})) \\
& \quad \Big(8\,(d_{12}-d_{21})\,d_{22}^3\,\alpha_1^4\,\beta_0\,(1+\Upsilon_{k,m}) - (d_{12}+d_{21})\,\alpha_3\,\hat{\beta}_a\,\big(d_{22}\,\alpha_3+\hat{\beta}_a\big)\,(1+d_{22}\,\alpha_3\,\beta_0\,(1+\Upsilon_{k,m})) + \\
& \qquad 2\,d_{22}^2\,\alpha_1^3\,\Big(d_{12}\,\big(1+8\,d_{22}\,\alpha_3\,\beta_0\,(1+\Upsilon_{k,m}) + 5\,\beta_0\,\hat{\beta}_a\,(1+\Upsilon_{k,m})\big) - \\
& \qquad\quad d_{21}\,\big(5+12\,d_{22}\,\alpha_3\,\beta_0\,(1+\Upsilon_{k,m}) + 5\,\beta_0\,\hat{\beta}_a\,(1+\Upsilon_{k,m})\big)\Big) + \\
& \qquad \alpha_1\,\Big(-3\,(d_{12}+d_{21})\,\hat{\beta}_a^2 + (5\,d_{12}-7\,d_{21})\,d_{22}^3\,\alpha_3^3\,\beta_0\,(1+\Upsilon_{k,m}) - \\
& \qquad\quad d_{22}\,\alpha_3\,\hat{\beta}_a\,\Big(d_{12}\,\big(4+\beta_0\,\hat{\beta}_a\,(1+\Upsilon_{k,m})\big) + d_{21}\,\big(4+5\,\beta_0\,\hat{\beta}_a\,(1+\Upsilon_{k,m})\big)\Big) + d_{22}^2\,\alpha_3^2 \\
& \qquad\quad \Big(d_{12}\,\big(5+2\,\beta_0\,\hat{\beta}_a\,(1+\Upsilon_{k,m})\big) - d_{21}\,\big(7+10\,\beta_0\,\hat{\beta}_a\,(1+\Upsilon_{k,m})\big)\Big)\Big) + d_{22}\,\alpha_1^2\,\Big(3\,(5\,d_{12}-7\,d_{21}) \\
& \qquad\quad d_{22}^2\,\alpha_3^2\,\beta_0\,(1+\Upsilon_{k,m}) + \hat{\beta}_a\,\Big(d_{12}\,\big(-7+2\,\beta_0\,\hat{\beta}_a\,(1+\Upsilon_{k,m})\big) - d_{21}\,\big(7+2\,\beta_0\,\hat{\beta}_a\,(1+\Upsilon_{k,m})\big)\Big) + \\
& \qquad\quad d_{22}\,\alpha_3\,\Big(9\,d_{12}\,\big(1+\beta_0\,\hat{\beta}_a\,(1+\Upsilon_{k,m})\big) - d_{21}\,\big(15+23\,\beta_0\,\hat{\beta}_a\,(1+\Upsilon_{k,m})\big)\Big)\Big)\Big)\Big)
\end{aligned}
$$

---

$$
\begin{aligned}
p_{2\,(2)} = {} & \Bigg((d_{12}+d_{21})\,\Bigg(-3\,q_1\,\alpha_3 + \frac{\hat{\chi}\,\alpha_1\,\alpha_2\,\big(d_{22}\,(4\,\alpha_1+3\,\alpha_3)+\hat{\beta}_a\big)\,(1+d_{22}\,\alpha_3\,\beta_0\,(1+\Upsilon_{k,m}))}{d_{22}\,(\alpha_1+\alpha_3)^2\,\big(d_{22}\,\alpha_1+\hat{\beta}_a\big)} - \\
& \quad \frac{q_2\,\alpha_3\,\big(3\,\alpha_3+3\,d_{22}\,\alpha_1^2\,\beta_0\,(1+\Upsilon_{k,m}) + \alpha_1\,(1+d_{22}\,\alpha_3\,\beta_0\,(1+\Upsilon_{k,m}))\big)}{\alpha_1+\alpha_3}\Bigg)\Bigg)\Big/\Big(2 \\
& \quad (1+d_{22}\,\alpha_3\,\beta_0\,(1+\Upsilon_{k,m}))^2\Big)
\end{aligned}
$$

---

$$p_{3\,(2)} = \frac{1}{2\,(1 + d_{22}\,\alpha_3\,\beta_0\,(1 + \Upsilon_{k,m}))^2}\left(\frac{\hat{\chi}\,\alpha_1\,\alpha_2\,\left(-d_{11}\,d_{22}\,\alpha_3 + d_{22}^2\,(\alpha_1+\alpha_3) + d_{11}\,\hat{\beta}_a\right)\,(1 + d_{22}\,\alpha_3\,\beta_0\,(1+\Upsilon_{k,m}))}{d_{22}\,(\alpha_1+\alpha_3)^2\,\left(d_{22}\,\alpha_1 + \hat{\beta}_a\right)} + q_1\,\alpha_3\,(d_{11} + d_{22}\,(-1 + 2\,d_{22}\,\alpha_3\,\beta_0\,r_{1,m}\,\Upsilon_{k,m})) + \frac{q_2\,(\alpha_1-\alpha_3)\,\left(-d_{11}\,\alpha_3 - 2\,d_{22}^2\,\alpha_3\,(\alpha_1+\alpha_3)\,\beta_0\,r_{1,m}\,\Upsilon_{k,m} + d_{22}\,(\alpha_3 + \alpha_1\,(1 + d_{11}\,\alpha_3\,\beta_0\,(1+\Upsilon_{k,m})))\right)}{\alpha_1+\alpha_3}\right)$$

---

$$\begin{aligned}
p_{4\,(4)} = {} & \frac{1}{4\,(1 + d_{22}\,\alpha_3\,\beta_0\,(1 + \Upsilon_{k,m}))^3}\,(d_{12} + d_{21}) \\
& \Bigl(q_1\,\alpha_3\,\bigl(-3 - 6\,\beta_0\,r_{1,m} + \beta_0\,(3 + 6\,r_{1,m} + d_{22}\,\alpha_3\,(-3 + 2\,\beta_0\,r_{1,m}))\,(1 + \Upsilon_{k,m}) + {} \\
& \quad \alpha_3\,\beta_0^2\,(4\,d_{11} - d_{22}\,(1 + 2\,r_{1,m}))\,(1 + \Upsilon_{k,m})^2\bigr) - 1\big/\bigl(d_{22}\,(\alpha_1 + \alpha_3)^2\bigr)\,q_2\,\alpha_3\,\bigl(d_{22}\,\alpha_1\,\alpha_3 \\
& \quad \bigl(4 + 8\,\beta_0\,r_{1,m} + \beta_0\,(-4 + 5\,d_{22}\,\alpha_3 - 8\,r_{1,m})\,(1 + \Upsilon_{k,m}) + \alpha_3\,(-4\,d_{11} + d_{22}^2\,\alpha_3)\,\beta_0^2\,(1 + \Upsilon_{k,m})^2\bigr) + {} \\
& \quad \alpha_1^2\,\bigl(d_{22} + 2\,d_{22}\,\beta_0\,r_{1,m} + \beta_0\,(4\,d_{11} + d_{22}\,(-1 - 2\,r_{1,m} + 5\,d_{22}\,\alpha_3\,(1 + 2\,\beta_0\,r_{1,m})))\,(1 + \Upsilon_{k,m}) + {} \\
& \quad\quad d_{22}\,\alpha_3\,\beta_0^2\,(8\,d_{11} + d_{22}\,(-5 + 4\,d_{22}\,\alpha_3 - 10\,r_{1,m}))\,(1 + \Upsilon_{k,m})^2\bigr) + {} \\
& \quad d_{22}\,\alpha_3^2\,\bigl(3 + 6\,\beta_0\,r_{1,m} - \beta_0\,(3 + 6\,r_{1,m} + d_{22}\,\alpha_3\,(-3 + 2\,\beta_0\,r_{1,m}))\,(1 + \Upsilon_{k,m}) + {} \\
& \quad\quad \alpha_3\,\beta_0^2\,(-4\,d_{11} + d_{22}\,(1 + 2\,r_{1,m}))\,(1 + \Upsilon_{k,m})^2\bigr) + d_{22}^2\,\alpha_1^3\,\beta_0\,(1 + \Upsilon_{k,m}) \\
& \quad \bigl(3 - 4\,d_{11}\,\alpha_3\,\beta_0^2\,(1 + \Upsilon_{k,m})^2 + \beta_0\,(3\,d_{22}\,\alpha_3\,(1 + \Upsilon_{k,m}) - 4\,(1 + (1 + 2\,r_{1,m})\,\Upsilon_{k,m}))\bigr)\bigr) + {} \\
& 1\big/\bigl(d_{22}\,(\alpha_1 + \alpha_3)^2\,(d_{22}\,\alpha_1 + \hat{\beta}_a)^2\bigr)\,\hat{\chi}\,\alpha_1\,\alpha_2\,(1 + d_{22}\,\alpha_3\,\beta_0\,(1 + \Upsilon_{k,m})) \\
& \bigl(d_{22}^2\,\alpha_1^2\,\bigl(4 + 8\,\beta_0\,r_{1,m} + 4\,\beta_0\,(-1 + d_{22}\,\alpha_3 - 2\,r_{1,m})\,(1 + \Upsilon_{k,m}) + (-4\,d_{11} + d_{22})\,\alpha_3\,\beta_0^2\,(1 + \Upsilon_{k,m})^2\bigr) + {} \\
& \quad \hat{\beta}_a\,\bigl(-3\,d_{22}^2\,\alpha_3^2\,\beta_0\,(1 + \Upsilon_{k,m})\,(-1 + \beta_0\,(1 + \Upsilon_{k,m})) + \alpha_3\,\bigl(3\,d_{22}\,(1 + 2\,\beta_0\,r_{1,m}) + \beta_0 \\
& \quad\quad \bigl(4\,d_{11} + d_{22}\,(-7 + \hat{\beta}_a - 6\,r_{1,m})\bigr)\,(1 + \Upsilon_{k,m})\bigr) - \hat{\beta}_a\,(-1 + \beta_0\,(1 + (1 + 2\,r_{1,m})\,\Upsilon_{k,m}))\bigr) + {} \\
& \quad \alpha_1\,\bigl(d_{22}^2\,\alpha_3^2\,\beta_0\,(1 + \Upsilon_{k,m})\,(3\,d_{22} + (-4\,d_{11} + d_{22})\,\beta_0\,(1 + \Upsilon_{k,m})) + {} \\
& \quad\quad d_{22}^2\,\alpha_3\,\bigl(3 - 3\,\beta_0^2\,\hat{\beta}_a\,(1 + \Upsilon_{k,m})^2 + \beta_0\,\bigl(5\,\hat{\beta}_a\,(1 + \Upsilon_{k,m}) - 3\,(1 + (1 + 2\,r_{1,m})\,\Upsilon_{k,m})\bigr)\bigr) + {} \\
& \quad\quad \hat{\beta}_a\,(4\,d_{11}\,\beta_0\,(1 + \Upsilon_{k,m}) - d_{22}\,(-5 + \beta_0\,(9 + (9 + 10\,r_{1,m})\,\Upsilon_{k,m})))\bigr)\bigr)\Bigr)
\end{aligned}$$

---

$$p_{5\,(4)} = \frac{1}{8\, d_{22}^2\, (1 + d_{22}\,\alpha_3\,\beta_0\,(1 + \Upsilon_{k,m}))^3} \Big(d_{22}\, q_1\, \alpha_3$$

$$\Big(-d_{22}\Big(-2\, d_{11}\,(1 + 2\,\beta_0\, r_{1,m}) + d_{22}\Big(3 + 8\, d_{22}\,\alpha_3\,\beta_0^2\, r_{1,m}^2 + 4\,\beta_0\,((1 + d_{22}\,\alpha_3)\, r_{1,m} + 2\, r_{2,m})\Big)\Big) -$$

$$\beta_0\Big(d_{11}^2 + 2\, d_{11}\, d_{22}\,(1 + 2\, r_{1,m} + d_{22}\,\alpha_3\,(-1 + 2\,\beta_0\, r_{1,m})) + d_{22}^2\Big(-3 - 4\, r_{1,m} + 4\, d_{22}^2\,\alpha_3^2\,\beta_0\, r_{1,m} -$$

$$8\, r_{2,m} - 4\, d_{22}\,\alpha_3\Big(-1 + (1 + \beta_0)\, r_{1,m} + 4\,\beta_0\, r_{1,m}^2 - 2\,\beta_0\, r_{2,m}\Big)\Big)\Big)\,(1 + \Upsilon_{k,m}) + d_{22}\,\alpha_3\,\beta_0^2$$

$$\Big(-3\, d_{11}^2 + 2\, d_{11}\, d_{22}\,(1 + 2\, r_{1,m}) + d_{22}^2\Big(1 - 4\, r_{1,m} - 8\, r_{1,m}^2 + d_{22}\,\alpha_3\,(-1 + 4\, r_{1,m}) + 8\, r_{2,m}\Big)\Big)$$

$$(1 + \Upsilon_{k,m})^2\Big) - 1\Big/(\alpha_1 + \alpha_3)^2\, d_{22}\, q_2\,(\alpha_1 - \alpha_3)\Big(\alpha_3^2\Big(-d_{22}$$

$$\Big(-2\, d_{11}\,(1 + 2\,\beta_0\, r_{1,m}) + d_{22}\Big(3 + 8\, d_{22}\,\alpha_3\,\beta_0^2\, r_{1,m}^2 + 4\,\beta_0\,((1 + d_{22}\,\alpha_3)\, r_{1,m} + 2\, r_{2,m})\Big)\Big) -$$

$$\beta_0\Big(d_{11}^2 + 2\, d_{11}\, d_{22}\,(1 + 2\, r_{1,m} + d_{22}\,\alpha_3\,(-1 + 2\,\beta_0\, r_{1,m})) + d_{22}^2\Big(-3 - 4\, r_{1,m} +$$

$$4\, d_{22}^2\,\alpha_3^2\,\beta_0\, r_{1,m} - 8\, r_{2,m} - 4\, d_{22}\,\alpha_3\Big(-1 + (1 + \beta_0)\, r_{1,m} + 4\,\beta_0\, r_{1,m}^2 - 2\,\beta_0\, r_{2,m}\Big)\Big)\Big)$$

$$(1 + \Upsilon_{k,m}) + d_{22}\,\alpha_3\,\beta_0^2\Big(-3\, d_{11}^2 + 2\, d_{11}\, d_{22}\,(1 + 2\, r_{1,m}) + d_{22}^2\Big(1 - 4\, r_{1,m} -$$

$$8\, r_{1,m}^2 + d_{22}\,\alpha_3\,(-1 + 4\, r_{1,m}) + 8\, r_{2,m}\Big)\Big)\,(1 + \Upsilon_{k,m})^2\Big) + \alpha_1\,\alpha_3\Big(-2\, d_{22}$$

$$\Big(-d_{11}\,(1 + 2\,\beta_0\, r_{1,m}) + d_{22}\Big(3 + 8\, d_{22}\,\alpha_3\,\beta_0^2\, r_{1,m}^2 + 4\,\beta_0\,((1 + d_{22}\,\alpha_3)\, r_{1,m} + 2\, r_{2,m})\Big)\Big) +$$

$$\beta_0\Big(-3\, d_{11}^2 - 2\, d_{11}\, d_{22}\,(1 + (2 + 6\, d_{22}\,\alpha_3\,\beta_0)\, r_{1,m}) + 2\, d_{22}^2\Big(3 + 4\, r_{1,m} - 4\, d_{22}^2\,\alpha_3^2\,\beta_0\, r_{1,m} +$$

$$8\, r_{2,m} + 4\, d_{22}\,\alpha_3\Big(-1 + (1 + \beta_0)\, r_{1,m} + 4\,\beta_0\, r_{1,m}^2 - 2\,\beta_0\, r_{2,m}\Big)\Big)\Big)\,(1 + \Upsilon_{k,m}) -$$

$$2\, d_{22}\,\alpha_3\,\beta_0^2\Big(3\, d_{11}^2 + d_{11}\, d_{22}\,(-3 + d_{22}\,\alpha_3 - 6\, r_{1,m}) + d_{22}^2\Big(-1 + d_{22}\,\alpha_3\,(1 - 4\, r_{1,m}) +$$

$$4\, r_{1,m} + 8\, r_{1,m}^2 - 8\, r_{2,m}\Big)\Big)\,(1 + \Upsilon_{k,m})^2 + d_{11}^2\, d_{22}^2\,\alpha_3^2\,\beta_0^3\,(1 + \Upsilon_{k,m})^3\Big) +$$

$$d_{22}\,\alpha_1^2\Big(\alpha_3\,\beta_0\Big(-4\, d_{22}^2\, r_{1,m}\,(1 + 2\,\beta_0\, r_{1,m}) - 2\, d_{22}\Big(d_{11}\,(1 + 4\,\beta_0\, r_{1,m}) -$$

$$2\, d_{22}\Big(-1 + (1 + \beta_0)\, r_{1,m} + 4\,\beta_0\, r_{1,m}^2 - 2\,\beta_0\, r_{2,m}\Big)\Big)\,(1 + \Upsilon_{k,m}) +$$

$$\beta_0\Big(d_{11}^2 + 4\, d_{11}\, d_{22}\,(1 + 2\, r_{1,m}) + d_{22}^2\Big(1 - 4\, r_{1,m} - 8\, r_{1,m}^2 + 8\, r_{2,m}\Big)\Big)\,(1 + \Upsilon_{k,m})^2\Big) +$$

$$d_{22}\,\alpha_3^2\,\beta_0^2\,(1 + \Upsilon_{k,m})\Big(-2\, d_{11}\, d_{22}\,(1 + \Upsilon_{k,m}) + 3\, d_{11}^2\,\beta_0\,(1 + \Upsilon_{k,m})^2 +$$

$$d_{22}^2\,(-1 + (-1 + 4\, r_{1,m})\,\Upsilon_{k,m})\Big) + d_{22}\,(-3 + \beta_0\,(3 + (3 + 4\, r_{1,m} + 8\, r_{2,m})\,\Upsilon_{k,m}))\Big)\Big) +$$

$$1\Big/\Big((\alpha_1 + \alpha_3)^3\,\Big(d_{22}\,\alpha_1 + \hat{\beta}_a\Big)^2\Big)\,\hat{\chi}\,\alpha_1\,\alpha_2\,(1 + d_{22}\,\alpha_3\,\beta_0\,(1 + \Upsilon_{k,m}))$$

$$\Big(-d_{22}^4\,\alpha_1^3\Big(-2 - 4\,\beta_0\, r_{1,m} + \beta_0\,(3 - 2\, d_{22}\,\alpha_3 + 4\, r_{1,m})\,(1 + \Upsilon_{k,m}) + (2\, d_{11} + d_{22})\,\alpha_3\,\beta_0^2\,(1 + \Upsilon_{k,m})^2\Big) +$$

$$\alpha_3\,\hat{\beta}_a\Big((d_{11} - d_{22})\, d_{22}^2\,\alpha_3^2\,\beta_0\,(1 + \Upsilon_{k,m})\,(-2\, d_{22} + (d_{11} + 3\, d_{22})\,\beta_0\,(1 + \Upsilon_{k,m})) -$$

$$d_{22}\,\alpha_3\Big(2\,(d_{11} - d_{22})\, d_{22}\,(1 + 2\,\beta_0\, r_{1,m}) + \beta_0\Big(d_{11}^2 - 2\, d_{11}\, d_{22}\Big(3 + \hat{\beta}_a + 2\, r_{1,m}\Big) +$$

$$d_{22}^2\,(5 + 4\, r_{1,m})\Big)\,(1 + \Upsilon_{k,m}) + d_{11}^2\,\beta_0^2\,\hat{\beta}_a\,(1 + \Upsilon_{k,m})^2\Big) +$$

$$d_{11}\,\hat{\beta}_a\,(d_{11}\,\beta_0\,(1 + \Upsilon_{k,m}) - 2\, d_{22}\,(-1 + \beta_0\,(1 + (1 + 2\, r_{1,m})\,\Upsilon_{k,m})))\Big) +$$

$$\alpha_1\Big((d_{11} - d_{22})\, d_{22}^3\,\alpha_3^3\,\beta_0\,(1 + \Upsilon_{k,m})\,(-2\, d_{22} + (3\, d_{11} + d_{22})\,\beta_0\,(1 + \Upsilon_{k,m})) +$$

$$d_{22}\,\alpha_3\,\hat{\beta}_a\Big(4\, d_{22}^2\,(1 + 2\,\beta_0\, r_{1,m}) +$$

$$2\, d_{22}\,\beta_0\Big(d_{11}\Big(4 + \hat{\beta}_a\Big) - d_{22}\,(5 + 4\, r_{1,m})\Big)\,(1 + \Upsilon_{k,m}) - 3\, d_{11}^2\,\beta_0^2\,\hat{\beta}_a\,(1 + \Upsilon_{k,m})^2\Big) +$$

$$d_{22}^2\,\alpha_3^2\Big(-2\,(d_{11} - d_{22})\, d_{22}\,(1 + 2\,\beta_0\, r_{1,m}) + \beta_0\Big(d_{11}^2 + d_{22}^2\Big(-3 + 4\,\hat{\beta}_a - 4\, r_{1,m}\Big) +$$

$$2\, d_{11}\, d_{22}\,(1 + 2\, r_{1,m})\Big)\,(1 + \Upsilon_{k,m}) + 2\,(2\, d_{11} - 3\, d_{22})\, d_{22}\,\beta_0^2\,\hat{\beta}_a\,(1 + \Upsilon_{k,m})^2\Big) -$$

$$d_{11}\,\hat{\beta}_a^2\,(d_{11}\,\beta_0\,(1 + \Upsilon_{k,m}) + 2\, d_{22}\,(-1 + \beta_0\,(1 + (1 + 2\, r_{1,m})\,\Upsilon_{k,m})))\Big) +$$

$$d_{22}\,\alpha_1^2\Big(d_{22}^2\,\alpha_3^2\,\beta_0\,(1 + \Upsilon_{k,m})\Big(-2\,(d_{11} - 2\, d_{22})\, d_{22} + \Big(5\, d_{11}^2 - 4\, d_{11}\, d_{22} - 2\, d_{22}^2\Big)\,\beta_0\,(1 + \Upsilon_{k,m})\Big) +$$

$$d_{22}\,\alpha_3\Big(-2\,(d_{11} - 2\, d_{22})\, d_{22}\,(1 + 2\,\beta_0\, r_{1,m}) +$$

$$\beta_0\Big(3\, d_{11}^2 + 2\, d_{22}^2\Big(-3 + \hat{\beta}_a - 4\, r_{1,m}\Big) + 2\, d_{11}\, d_{22}\Big(1 + \hat{\beta}_a + 2\, r_{1,m}\Big)\Big)\,(1 + \Upsilon_{k,m}) +$$

$$\Big(-5\, d_{11}^2 + 2\, d_{11}\, d_{22} - 3\, d_{22}^2\Big)\,\beta_0^2\,\hat{\beta}_a\,(1 + \Upsilon_{k,m})^2\Big) + \hat{\beta}_a\Big(-3\, d_{11}^2\,\beta_0\,(1 + \Upsilon_{k,m}) +$$

$$2\, d_{11}\, d_{22}\,(1 + \beta_0\,(1 + (1 - 2\, r_{1,m})\,\Upsilon_{k,m})) - d_{22}^2\,(-2 + \beta_0\,(5 + (5 + 4\, r_{1,m})\,\Upsilon_{k,m}))\Big)\Big)\Big)\Big)$$

$$p_{6\,(4)} = \frac{1}{4\,d_{22}^2\,(1 + d_{22}\,\alpha_3\,\beta_0\,(1 + \Upsilon_{k,m}))^3}\,\beta_0$$

$$(1 + \Upsilon_{k,m})\,(d_{22}\,q_1\,(2\,(d_{12} - d_{21})\,d_{22}^2\,\alpha_3\,\beta_0\,(1 + (1 + 2\,r_{1,m})\,\Upsilon_{k,m}) +$$

$$d_{11}\,(d_{12}\,(1 - 5\,d_{22}\,\alpha_3\,\beta_0\,(1 + \Upsilon_{k,m})) - d_{21}\,(-1 + d_{22}\,\alpha_3\,\beta_0\,(1 + \Upsilon_{k,m})))) + 1 / (\alpha_1 + \alpha_3)^2\,d_{22}\,q_2$$

$$(d_{22}\,\alpha_1\,\alpha_3^2\,\beta_0\,(4\,(-d_{12} + d_{21})\,d_{22}\,r_{1,m} - (5\,d_{11}\,(d_{12} + d_{21}) - 2\,(d_{12} - d_{21})\,d_{22}\,(1 + 2\,r_{1,m}))$$

$$(1 + \Upsilon_{k,m}) + d_{11}\,(d_{12} - 3\,d_{21})\,d_{22}\,\alpha_3\,\beta_0\,(1 + \Upsilon_{k,m})^2) + d_{22}\,\alpha_1^3\,\beta_0$$

$$(4\,(d_{12} - d_{21})\,d_{22}\,r_{1,m} + (d_{11}\,(d_{12} + d_{21}) - 2\,(d_{12} - d_{21})\,d_{22}\,(1 + 2\,r_{1,m}))\,(1 + \Upsilon_{k,m}) - d_{11}$$

$$(5\,d_{12} + d_{21})\,d_{22}\,\alpha_3\,\beta_0\,(1 + \Upsilon_{k,m})^2) + \alpha_3^2\,(2\,(d_{12} - d_{21})\,d_{22}^2\,\alpha_3\,\beta_0\,(1 + (1 + 2\,r_{1,m})\,\Upsilon_{k,m}) +$$

$$d_{11}\,(d_{12}\,(1 - 5\,d_{22}\,\alpha_3\,\beta_0\,(1 + \Upsilon_{k,m})) - d_{21}\,(-1 + d_{22}\,\alpha_3\,\beta_0\,(1 + \Upsilon_{k,m})))) +$$

$$\alpha_1^2\,(-2\,(d_{12} - d_{21})\,d_{22}^2\,\alpha_3\,\beta_0\,(1 + (1 + 2\,r_{1,m})\,\Upsilon_{k,m}) +$$

$$d_{11}\,(d_{21}\,(11 + 21\,d_{22}\,\alpha_3\,\beta_0\,(1 + \Upsilon_{k,m}) + 8\,d_{22}^2\,\alpha_3^2\,\beta_0^2\,(1 + \Upsilon_{k,m})^2) +$$

$$d_{12}\,(11 + 25\,d_{22}\,\alpha_3\,\beta_0\,(1 + \Upsilon_{k,m}) + 8\,d_{22}^2\,\alpha_3^2\,\beta_0^2\,(1 + \Upsilon_{k,m})^2)))) -$$

$$1 / ((\alpha_1 + \alpha_3)^2\,(d_{22}\,\alpha_1 + \hat{\beta}_a)^2)\,(1 + d_{22}\,\alpha_3\,\beta_0\,(1 + \Upsilon_{k,m}))\,(2\,d_0\,(d_{12} + d_{21})\,d_{22}^4\,\alpha_1^4\,\alpha_3\,(1 + \epsilon_{s,m}) +$$

$$2\,d_{22}^3\,\alpha_1^3\,(2\,d_0\,(d_{12} + d_{21})\,d_{22}\,\alpha_3^2\,(1 + \epsilon_{s,m}) + 2\,d_0\,(d_{12} + d_{21})\,\alpha_3\,\hat{\beta}_a\,(1 + \epsilon_{s,m}) -$$

$$\hat{\chi}\,(2\,d_{11}\,(d_{12} + d_{21}) + (-d_{12} + d_{21})\,d_{22})\,\alpha_2\,\beta_0\,(1 + \Upsilon_{k,m})) +$$

$$(d_{12} + d_{21})\,\hat{\beta}_a\,(2\,d_0\,d_{22}^2\,\alpha_3^3\,\hat{\beta}_a\,(1 + \epsilon_{s,m}) + \hat{\chi}\,d_{11}\,\alpha_2\,(2\,d_{22}\,\alpha_3 + \hat{\beta}_a + d_{22}^2\,\alpha_3^2\,\beta_0\,(1 + \Upsilon_{k,m}))) +$$

$$d_{22}\,\alpha_1\,(4\,d_0\,(d_{12} + d_{21})\,d_{22}^2\,\alpha_3^3\,\hat{\beta}_a\,(1 + \epsilon_{s,m}) + d_{22}\,\alpha_3^2\,(4\,d_0\,(d_{12} + d_{21})\,\hat{\beta}_a^2\,(1 + \epsilon_{s,m}) +$$

$$\hat{\chi}\,d_{22}\,(-d_{11}\,(5\,d_{12} + d_{21}) + 2\,(d_{12} - d_{21})\,d_{22})\,\alpha_2\,\beta_0\,(1 + \Upsilon_{k,m})) +$$

$$2\,\hat{\chi}\,d_{22}\,(-2\,d_{11}\,d_{12} + (d_{12} - d_{21})\,d_{22})\,\alpha_2\,\alpha_3\,(1 + \beta_0\,\hat{\beta}_a\,(1 + \Upsilon_{k,m})) +$$

$$\hat{\chi}\,d_{11}\,\alpha_2\,\hat{\beta}_a\,(d_{21}\,(4 - 3\,\beta_0\,\hat{\beta}_a\,(1 + \Upsilon_{k,m})) + d_{12}\,(4 + \beta_0\,\hat{\beta}_a\,(1 + \Upsilon_{k,m})))) +$$

$$d_{22}^2\,\alpha_1^2\,(2\,d_0\,(d_{12} + d_{21})\,d_{22}^2\,\alpha_3^3\,(1 + \epsilon_{s,m}) + 8\,d_0\,(d_{12} + d_{21})\,d_{22}\,\alpha_3^2\,\hat{\beta}_a\,(1 + \epsilon_{s,m}) +$$

$$2\,\alpha_3\,(d_0\,(d_{12} + d_{21})\,\hat{\beta}_a^2\,(1 + \epsilon_{s,m}) + \hat{\chi}\,d_{22}\,(-d_{11}\,(5\,d_{12} + d_{21}) + 2\,(d_{12} - d_{21})\,d_{22})$$

$$\alpha_2\,\beta_0\,(1 + \Upsilon_{k,m})) + \hat{\chi}\,\alpha_2\,(2\,(d_{12} - d_{21})\,d_{22}\,(1 + \beta_0\,\hat{\beta}_a\,(1 + \Upsilon_{k,m})) +$$

$$d_{11}\,(d_{21}\,(1 - 7\,\beta_0\,\hat{\beta}_a\,(1 + \Upsilon_{k,m})) - 3\,d_{12}\,(1 + \beta_0\,\hat{\beta}_a\,(1 + \Upsilon_{k,m}))))))))$$

---

$$p_{7\,(4)} = \frac{1}{4\,d_{22}^2\,(\alpha_1 + \alpha_3)^3\,(d_{22}\,\alpha_1 + \hat{\beta}_a)^2\,(1 + d_{22}\,\alpha_3\,\beta_0\,(1 + \Upsilon_{k,m}))^3}$$

$$(d_{11}\,d_{22}^4\,q_2\,\alpha_1^6\,\beta_0\,(1 + \Upsilon_{k,m})\,(-d_{22}\,(1 + 4\,\beta_0\,r_{1,m}) + \beta_0\,(2\,d_{11} + d_{22}\,(2 - d_{22}\,\alpha_3 + 4\,r_{1,m}))\,(1 + \Upsilon_{k,m}) +$$

$$4\,d_{11}\,d_{22}\,\alpha_3\,\beta_0^2\,(1 + \Upsilon_{k,m})^2) + d_{22}^3\,\alpha_1^5\,(d_{11}\,(-d_{22}\,(q_1 - q_2)\,(1 + 2\,\beta_0\,r_{1,m}) -$$

$$\beta_0\,(-2\,d_{11}\,(q_1 - 4\,q_2) + d_{22}\,(-q_1\,(1 + 2\,r_{1,m}) + q_2\,(1 + 2\,r_{1,m} + \hat{\beta}_a\,(2 + 8\,\beta_0\,r_{1,m}))))$$

$$(1 + \Upsilon_{k,m}) + 4\,q_2\,\beta_0^2\,\hat{\beta}_a\,(d_{11} + d_{22}\,(1 + 2\,r_{1,m}))\,(1 + \Upsilon_{k,m})^2) -$$

$$2\,d_0\,d_{22}^4\,\alpha_3^3\,\beta_0^2\,(1 + \Upsilon_{k,m})^2\,(-1 + \epsilon_{s,m}\,(-1 + 2\,\beta_0\,r_{1,m}\,(1 + \Upsilon_{k,m})))) +$$

$$d_{22}^2\,\alpha_3^2\,\beta_0\,(1 + \Upsilon_{k,m})\,(-\beta_0\,(1 + \Upsilon_{k,m})\,(d_{11}\,d_{22}\,q_2 - 8\,d_0\,d_{22}\,r_{1,m} + 2\,d_{11}^2\,q_2\,\beta_0\,(1 + \Upsilon_{k,m})) +$$

$$2\,d_0\,(1 + \epsilon_{s,m})\,(2\,d_{22}\,(1 + \beta_0\,r_{1,m}) + \beta_0\,(d_{11} - d_{22}\,(1 + 6\,r_{1,m}))\,(1 + \Upsilon_{k,m}))) +$$

$$d_{22}\,\alpha_3\,(\beta_0\,(1 + \Upsilon_{k,m})\,(d_{22}\,(4\,d_0\,r_{1,m} + d_{11}\,(-6\,q_2\,\beta_0\,r_{1,m} + q_1\,(-1 + 2\,\beta_0\,r_{1,m}))) +$$

$$d_{11}\,\beta_0\,(2\,d_{11}\,(2\,q_1 - 7\,q_2) - d_{22}\,(q_2\,(-3 + 2\,\hat{\beta}_a - 6\,r_{1,m}) + q_1\,(1 + 2\,r_{1,m})))$$

$$(1 + \Upsilon_{k,m}) + 8\,d_{11}^2\,q_2\,\beta_0^2\,\hat{\beta}_a\,(1 + \Upsilon_{k,m})^2) +$$

$$2\, d_0\, (1+\epsilon_{s,m})\, (d_{11}\, \beta_0\, (1+\Upsilon_{k,m}) - d_{22}\, (-1+\beta_0\, (1+\Upsilon_{k,m}+r_{1,m}\, (2+4\, \Upsilon_{k,m})))))\big)\big) -$$

$$\alpha_3\, \hat{\beta}_a\, \big(\hat{\chi}\, d_{11}\, d_{22}\, \alpha_2\, \alpha_3\, \big(-d_{22}\, (1+2\, \beta_0\, r_{1,m}) + \beta_0\, \big(d_{11} - 2\, d_{22}\, \big(-1 - r_{1,m} + \hat{\beta}_a\, (1+\beta_0\, r_{1,m})\big)\big)\big)$$

$$(1+\Upsilon_{k,m}) + \beta_0^2\, \hat{\beta}_a\, (5\, d_{11} + d_{22}\, (1+2\, r_{1,m}))\, (1+\Upsilon_{k,m})^2\big) +$$

$$d_{11}\, d_{22}\, \alpha_3^2\, \big(d_{22}\, (q_1+q_2)\, \hat{\beta}_a\, (1+2\, \beta_0\, r_{1,m}) - \beta_0\, \big(2\, \hat{\chi}\, d_{22}^2\, \alpha_2\, (1+\beta_0\, r_{1,m}) +$$

$$(q_1+q_2)\, \hat{\beta}_a\, (2\, d_{11} + d_{22}\, (1+2\, r_{1,m}))\big)\, (1+\Upsilon_{k,m}) +$$

$$\hat{\chi}\, d_{22}\, \alpha_2\, \beta_0^2\, \big(3\, d_{11} + d_{22}\, \big(3 - \hat{\beta}_a + 2\, r_{1,m}\big)\big)\, (1+\Upsilon_{k,m})^2 + 3\, \hat{\chi}\, d_{11}\, d_{22}\, \alpha_2\, \beta_0^3\, \hat{\beta}_a\, (1+\Upsilon_{k,m})^3\big) +$$

$$2\, d_0\, d_{22}^5\, \alpha_3^5\, \beta_0^2\, \hat{\beta}_a\, (1+\Upsilon_{k,m})^2\, (-1+\epsilon_{s,m}\, (-1+2\, \beta_0\, r_{1,m}\, (1+\Upsilon_{k,m}))) -$$

$$2\, d_0\, d_{22}^3\, \alpha_3^4\, \beta_0\, \hat{\beta}_a\, (1+\Upsilon_{k,m})\, (4\, d_{22}\, \beta_0\, r_{1,m}\, (1+\Upsilon_{k,m}) +$$

$$(1+\epsilon_{s,m})\, (2\, d_{22}\, (1+\beta_0\, r_{1,m}) + \beta_0\, (d_{11} - d_{22}\, (1+6\, r_{1,m}))\, (1+\Upsilon_{k,m}))) +$$

$$\hat{\chi}\, d_{11}\, \alpha_2\, \hat{\beta}_a\, (2\, d_{11}\, \beta_0\, (1+\Upsilon_{k,m}) + d_{22}\, (-1+\beta_0\, (1+(1+2\, r_{1,m})\, \Upsilon_{k,m}))) +$$

$$d_{22}^2\, \alpha_3^3\, \big(\beta_0\, (1+\Upsilon_{k,m})\, \big(d_{22}\, \hat{\beta}_a\, (-4\, d_0\, r_{1,m} - d_{11}\, (q_1+q_2)\, (-1+2\, \beta_0\, r_{1,m})) +$$

$$d_{11}\, \beta_0\, \big(-\hat{\chi}\, d_{22}^2\, \alpha_2 - (q_1+q_2)\, \hat{\beta}_a\, (4\, d_{11} - d_{22}\, (1+2\, r_{1,m}))\big)\, (1+\Upsilon_{k,m}) +$$

$$\hat{\chi}\, d_{11}\, d_{22}\, (2\, d_{11} + d_{22})\, \alpha_2\, \beta_0^2\, (1+\Upsilon_{k,m})^2\big) -$$

$$2\, d_0\, \hat{\beta}_a\, (1+\epsilon_{s,m})\, (d_{11}\, \beta_0\, (1+\Upsilon_{k,m}) - d_{22}\, (-1+\beta_0\, (1+\Upsilon_{k,m}+r_{1,m}\, (2+4\, \Upsilon_{k,m})))))\big) +$$

$$d_{22}^2\, \alpha_1^4\, \big(d_{11}\, \big(-2\, d_{22}\, (q_1-q_2)\, \hat{\beta}_a\, (1+2\, \beta_0\, r_{1,m}) - \beta_0\, \hat{\beta}_a\, \big(-4\, d_{11}\, (q_1-4\, q_2) +$$

$$d_{22}\, \big(-2\, q_1\, (1+2\, r_{1,m}) + q_2\, \big(2+4\, r_{1,m}+\hat{\beta}_a\, (1+4\, \beta_0\, r_{1,m})\big)\big)\big)\big)\, (1+\Upsilon_{k,m}) +$$

$$\beta_0^2\, \big(\hat{\chi}\, d_{22}^2\, \alpha_2 + 2\, q_2\, \hat{\beta}_a^2\, (d_{11} + d_{22}\, (1+2\, r_{1,m}))\big)\, (1+\Upsilon_{k,m})^2\big) -$$

$$6\, d_0\, d_{22}^5\, \alpha_3^4\, \beta_0^2\, (1+\Upsilon_{k,m})^2\, (-1+\epsilon_{s,m}\, (-1+2\, \beta_0\, r_{1,m}\, (1+\Upsilon_{k,m}))) +$$

$$d_{22}^2\, \alpha_3^2\, \big(-\beta_0\, (1+\Upsilon_{k,m})\, \big(-d_{22}\, (12\, d_0\, r_{1,m} + d_{11}\, (2\, q_2\, (1+\beta_0\, r_{1,m}) + q_1\, (-3+6\, \beta_0\, r_{1,m}))) +$$

$$\beta_0\, \big(6\, d_{11}^2\, (-2\, q_1+q_2) - 16\, d_0\, d_{22}\, \hat{\beta}_a\, r_{1,m} + d_{11}\, d_{22}\, \big(q_2\, \big(1+2\, \hat{\beta}_a+2\, r_{1,m}\big) +$$

$$q_1\, (3+6\, r_{1,m})\big)\big)\, (1+\Upsilon_{k,m}) + 4\, d_{11}^2\, q_2\, \beta_0^2\, \hat{\beta}_a\, (1+\Upsilon_{k,m})^2\big) + 2\, d_0\, (1+\epsilon_{s,m})$$

$$\big(3\, d_{22}\, (1+2\, \beta_0\, r_{1,m}) + \beta_0\, \big(3\, d_{11} + d_{22}\, \big(-3\, (1+4\, r_{1,m}) + 4\, \hat{\beta}_a\, (1+\beta_0\, r_{1,m})\big)\big)$$

$$(1+\Upsilon_{k,m}) + 2\, \beta_0^2\, \hat{\beta}_a\, (d_{11} - d_{22}\, (1+6\, r_{1,m}))\, (1+\Upsilon_{k,m})^2\big)\big) +$$

$$d_{22}^3\, \alpha_3^3\, \beta_0\, (1+\Upsilon_{k,m})\, \big(2\, d_0\, (1+\epsilon_{s,m})\, \big(6\, d_{22}\, (1+\beta_0\, r_{1,m}) + \beta_0\, \big(3\, d_{11} +$$

$$d_{22}\, \big(-3+2\, \hat{\beta}_a-18\, r_{1,m}\big)\big)\big)\, (1+\Upsilon_{k,m}) - 4\, d_{22}\, \beta_0^2\, \hat{\beta}_a\, r_{1,m}\, (1+\Upsilon_{k,m})^2\big) +$$

$$\beta_0\, (1+\Upsilon_{k,m})\, \big(d_{11}\, d_{22}\, q_2 - 4\, d_{11}^2\, q_2\, \beta_0\, (1+\Upsilon_{k,m}) + 8\, d_0\, d_{22}\, r_{1,m}\, \big(3+\beta_0\, \hat{\beta}_a\, (1+\Upsilon_{k,m})\big)\big)\big) +$$

$$d_{22}\, \alpha_3\, \big(-d_{11}\, d_{22}\, (3\, q_1-q_2)\, (1+2\, \beta_0\, r_{1,m}) + \beta_0\, \big(d_{11}^2\, (6\, q_1-2\, q_2) + 8\, d_0\, d_{22}\, \hat{\beta}_a\, r_{1,m} + d_{11}\, d_{22}$$

$$\big(-q_2\, \big(1+2\, \big(1+6\, \beta_0\, \hat{\beta}_a\big)\, r_{1,m}\big) + q_1\, \big(3+6\, r_{1,m}+\hat{\beta}_a\, (-2+4\, \beta_0\, r_{1,m})\big)\big)\big)\, (1+\Upsilon_{k,m}) +$$

$$d_{11}\, \beta_0^2\, \hat{\beta}_a\, \big(4\, d_{11}\, (2\, q_1-7\, q_2) - d_{22}\, \big(q_2\, \big(-6+\hat{\beta}_a-12\, r_{1,m}\big) + q_1\, (2+4\, r_{1,m})\big)\big)$$

$$(1+\Upsilon_{k,m})^2 + d_{11}\, \beta_0^3\, \big(\hat{\chi}\, d_{22}^2\, \alpha_2 + 4\, d_{11}\, q_2\, \hat{\beta}_a^2\big)\, (1+\Upsilon_{k,m})^3 +$$

$$4\, d_0\, \hat{\beta}_a\, (1+\epsilon_{s,m})\, (d_{11}\, \beta_0\, (1+\Upsilon_{k,m}) - d_{22}\, (-1+\beta_0\, (1+\Upsilon_{k,m}+r_{1,m}\, (2+4\, \Upsilon_{k,m})))))\big)\big) +$$

$$d_{22}\, \alpha_1^3\, \big(d_{11}\, \big(d_{22}\, \big(2\, \hat{\chi}\, d_{22}\, \alpha_2 + (-q_1+q_2)\, \hat{\beta}_a^2\big)\, (1+2\, \beta_0\, r_{1,m}) +$$

$$\beta_0\, \big(\hat{\beta}_a^2\, (2\, d_{11}\, (q_1-4\, q_2) + d_{22}\, (q_1-q_2)\, (1+2\, r_{1,m})) - \hat{\chi}\, d_{22}\, \alpha_2$$

$$(11\, d_{11} + d_{22}\, (1+4\, r_{1,m}))\big)\, (1+\Upsilon_{k,m}) + \hat{\chi}\, d_{22}\, (d_{11}+d_{22})\, \alpha_2\, \beta_0^2\, \hat{\beta}_a\, (1+\Upsilon_{k,m})^2\big) -$$

$$6\, d_0\, d_{22}^6\, \alpha_3^5\, \beta_0^2\, (1+\Upsilon_{k,m})^2\, (-1+\epsilon_{s,m}\, (-1+2\, \beta_0\, r_{1,m}\, (1+\Upsilon_{k,m}))) +$$

$$d_{22}^2\, \alpha_3^2\, \big(-d_{11}\, d_{22}\, (3\, q_1+q_2)\, (1+2\, \beta_0\, r_{1,m}) + \beta_0\, \big(d_{11}^2\, (6\, q_1+8\, q_2) + 24\, d_0\, d_{22}\, \hat{\beta}_a\, r_{1,m} + d_{11}\, d_{22}$$

$$\big(q_2\, \big(1+2\, r_{1,m}+4\, \hat{\beta}_a\, (1+\beta_0\, r_{1,m})\big) + 3\, q_1\, \big(1+2\, r_{1,m}+\hat{\beta}_a\, (-2+4\, \beta_0\, r_{1,m})\big)\big)\big)$$

$$(1+\Upsilon_{k,m}) + \beta_0^2\, \big(2\, \hat{\chi}\, d_{11}\, d_{22}^2\, \alpha_2 - \hat{\beta}_a\, \big(12\, d_{11}^2\, (-2\, q_1+q_2) - 8\, d_0\, d_{22}\, \hat{\beta}_a\, r_{1,m} +$$

$$d_{11} d_{22} (6 q_1 (1 + 2 r_{1,m}) + q_2 (2 + \hat{\beta}_a + 4 r_{1,m})))) (1 + \Upsilon_{k,m})^2 +$$

$$d_{11} \beta_0^3 (\hat{\chi} d_{22} (-14 d_{11} + 3 d_{22}) \alpha_2 - 2 d_{11} q_2 \hat{\beta}_a^2) (1 + \Upsilon_{k,m})^3 + 2 d_0 \hat{\beta}_a (1 + \epsilon_{s,m})$$

$$(6 d_{22} (1 + 2 \beta_0 r_{1,m}) + 2 \beta_0 (3 d_{11} + d_{22} (-3 (1 + 4 r_{1,m}) + \hat{\beta}_a (1 + \beta_0 r_{1,m})))$$

$$(1 + \Upsilon_{k,m}) + \beta_0^2 \hat{\beta}_a (d_{11} - d_{22} (1 + 6 r_{1,m})) (1 + \Upsilon_{k,m})^2)) +$$

$$d_{22}^3 \alpha_3^3 (\beta_0 (1 + \Upsilon_{k,m}) (3 d_{22} (4 d_0 r_{1,m} + d_{11} (2 q_2 \beta_0 r_{1,m} + q_1 (-1 + 2 \beta_0 r_{1,m})))) +$$

$$\beta_0 (2 d_{11}^2 (6 q_1 + 7 q_2) + 48 d_0 d_{22} \hat{\beta}_a r_{1,m} -$$

$$d_{11} d_{22} (q_1 (3 + 6 r_{1,m}) + q_2 (3 - 2 \hat{\beta}_a + 6 r_{1,m}))) (1 + \Upsilon_{k,m}) +$$

$$4 \beta_0^2 \hat{\beta}_a (-2 d_{11}^2 q_2 + d_0 d_{22} \hat{\beta}_a r_{1,m}) (1 + \Upsilon_{k,m})^2) + 2 d_0 (1 + \epsilon_{s,m})$$

$$(3 d_{22} (1 + 2 \beta_0 r_{1,m}) + 3 \beta_0 (d_{11} + d_{22} (-1 - 4 r_{1,m} + 4 \hat{\beta}_a (1 + \beta_0 r_{1,m}))) (1 + \Upsilon_{k,m}) +$$

$$\beta_0^2 \hat{\beta}_a (6 d_{11} + d_{22} (-6 + \hat{\beta}_a - 36 r_{1,m})) (1 + \Upsilon_{k,m})^2 - 2 d_{22} \beta_0^3 \hat{\beta}_a^2 r_{1,m} (1 + \Upsilon_{k,m})^3)) +$$

$$d_{22}^4 \alpha_3^4 \beta_0 (1 + \Upsilon_{k,m}) (-6 d_0 (1 + \epsilon_{s,m}) (-2 d_{22} (1 + \beta_0 r_{1,m}) +$$

$$\beta_0 (-d_{11} + d_{22} (1 - 2 \hat{\beta}_a + 6 r_{1,m})) (1 + \Upsilon_{k,m}) + 4 d_{22} \beta_0^2 \hat{\beta}_a r_{1,m} (1 + \Upsilon_{k,m})^2) +$$

$$\beta_0 (1 + \Upsilon_{k,m}) (d_{11} d_{22} q_2 + 2 d_{11}^2 q_2 \beta_0 (1 + \Upsilon_{k,m}) + 24 d_0 d_{22} r_{1,m} (1 + \beta_0 \hat{\beta}_a (1 + \Upsilon_{k,m})))) +$$

$$d_{22} \alpha_3 (-2 d_{11} d_{22} (3 q_1 - q_2) \hat{\beta}_a (1 + 2 \beta_0 r_{1,m}) +$$

$$\beta_0 (4 \hat{\chi} d_{11} d_{22}^2 \alpha_2 (1 + \beta_0 r_{1,m}) + \hat{\beta}_a (4 d_{11}^2 (3 q_1 - q_2) + 4 d_0 d_{22} \hat{\beta}_a r_{1,m} + d_{11} d_{22}$$

$$(-2 q_2 (1 + (2 + 3 \beta_0 \hat{\beta}_a) r_{1,m}) + q_1 (6 + 12 r_{1,m} + \hat{\beta}_a (-1 + 2 \beta_0 r_{1,m})))))$$

$$(1 + \Upsilon_{k,m}) + d_{11} \beta_0^2 (\hat{\chi} d_{22} \alpha_2 (-25 d_{11} + 2 d_{22} (1 - 2 r_{1,m})) +$$

$$\hat{\beta}_a^2 (2 d_{11} (2 q_1 - 7 q_2) - d_{22} (q_1 - 3 q_2) (1 + 2 r_{1,m}))) (1 + \Upsilon_{k,m})^2 +$$

$$\hat{\chi} d_{11} d_{22} (d_{11} + d_{22}) \alpha_2 \beta_0^3 \hat{\beta}_a (1 + \Upsilon_{k,m})^3 + 2 d_0 \hat{\beta}_a^2 (1 + \epsilon_{s,m})$$

$$(d_{11} \beta_0 (1 + \Upsilon_{k,m}) - d_{22} (-1 + \beta_0 (1 + \Upsilon_{k,m} + r_{1,m} (2 + 4 \Upsilon_{k,m}))))))) +$$

$$d_{22} \alpha_1^2 (d_{11} \alpha_3 (d_{22} (3 \hat{\chi} d_{22} \alpha_2 + (-3 q_1 + q_2) \hat{\beta}_a^2) (1 + 2 \beta_0 r_{1,m}) +$$

$$\beta_0 ((3 q_1 - q_2) \hat{\beta}_a^2 (2 d_{11} + d_{22} (1 + 2 r_{1,m})) -$$

$$\hat{\chi} d_{22} \alpha_2 (8 d_{11} + d_{22} (1 + 6 r_{1,m} - 6 \hat{\beta}_a (1 + \beta_0 r_{1,m})))) (1 + \Upsilon_{k,m}) -$$

$$\hat{\chi} d_{22} \alpha_2 \beta_0^2 \hat{\beta}_a (37 d_{11} + 3 d_{22} (1 + 2 r_{1,m})) (1 + \Upsilon_{k,m})^2 + \hat{\chi} d_{11} d_{22} \alpha_2 \beta_0^3 \hat{\beta}_a^2 (1 + \Upsilon_{k,m})^3) -$$

$$2 d_0 d_{22}^6 \alpha_3^6 \beta_0^2 (1 + \Upsilon_{k,m})^2 (-1 + \epsilon_{s,m} (-1 + 2 \beta_0 r_{1,m} (1 + \Upsilon_{k,m}))) +$$

$$2 d_0 d_{22}^4 \alpha_3^5 \beta_0 (1 + \Upsilon_{k,m})$$

$$(4 d_{22} \beta_0 r_{1,m} (1 + \Upsilon_{k,m}) (1 + 3 \beta_0 \hat{\beta}_a (1 + \Upsilon_{k,m})) + (1 + \epsilon_{s,m}) (2 d_{22} (1 + \beta_0 r_{1,m}) +$$

$$\beta_0 (d_{11} + d_{22} (-1 + 6 \hat{\beta}_a - 6 r_{1,m})) (1 + \Upsilon_{k,m}) - 12 d_{22} \beta_0^2 \hat{\beta}_a r_{1,m} (1 + \Upsilon_{k,m})^2)) +$$

$$d_{22}^2 \alpha_3^3 (-d_{11} d_{22} (q_1 + q_2) (1 + 2 \beta_0 r_{1,m}) + \beta_0 (2 d_{11}^2 (q_1 + q_2) + 24 d_0 d_{22} \hat{\beta}_a r_{1,m} +$$

$$d_{11} d_{22} (q_2 (1 + 2 (1 + 6 \beta_0 \hat{\beta}_a) r_{1,m}) + q_1 (1 + 2 r_{1,m} + 6 \hat{\beta}_a (-1 + 2 \beta_0 r_{1,m}))))$$

$$(1 + \Upsilon_{k,m}) + \beta_0^2 (4 d_{11}^2 (6 q_1 + 7 q_2) \hat{\beta}_a + 24 d_0 d_{22} \hat{\beta}_a^2 r_{1,m} +$$

$$d_{11} d_{22} (3 \hat{\chi} d_{22} \alpha_2 + q_2 \hat{\beta}_a^2 - 6 (q_1 + q_2) \hat{\beta}_a (1 + 2 r_{1,m}))) (1 + \Upsilon_{k,m})^2 +$$

$$d_{11} \beta_0^3 (3 \hat{\chi} d_{22} (-4 d_{11} + d_{22}) \alpha_2 - 4 d_{11} q_2 \hat{\beta}_a^2) (1 + \Upsilon_{k,m})^3 + 6 d_0 \hat{\beta}_a (1 + \epsilon_{s,m})$$

$$(2 d_{22} (1 + 2 \beta_0 r_{1,m}) + 2 \beta_0 (d_{11} + d_{22} (-1 - 4 r_{1,m} + \hat{\beta}_a (1 + \beta_0 r_{1,m}))) (1 + \Upsilon_{k,m}) +$$

$$\beta_0^2\,\hat{\beta}_a\,(d_{11}-d_{22}\,(1+6\,r_{1,m}))\,(1+\Upsilon_{k,m})^2\Big)\Big)+$$

$$d_{22}^3\,\alpha_3^4\,\Big(\beta_0\,(1+\Upsilon_{k,m})\,\Big(d_{22}\,(4\,d_0\,r_{1,m}+d_{11}\,(q_1+q_2)\,(-1+2\,\beta_0\,r_{1,m}))+\beta_0\,\Big(4\,d_{11}^2\,(q_1+q_2)+$$

$$48\,d_0\,d_{22}\,\hat{\beta}_a\,r_{1,m}-d_{11}\,d_{22}\,\Big(q_1\,(1+2\,r_{1,m})+q_2\,\Big(1-2\,\hat{\beta}_a+2\,r_{1,m}\Big)\Big)\Big)\,(1+\Upsilon_{k,m})+$$

$$4\,\beta_0^2\,\hat{\beta}_a\,\Big(d_{11}^2\,q_2+3\,d_0\,d_{22}\,\hat{\beta}_a\,r_{1,m}\Big)\,(1+\Upsilon_{k,m})^2\Big)-2\,d_0\,(1+\epsilon_{s,m})$$

$$\Big(-d_{22}\,(1+2\,\beta_0\,r_{1,m})+\beta_0\,\Big(-d_{11}+d_{22}\,\Big(1+4\,r_{1,m}-12\,\hat{\beta}_a\,(1+\beta_0\,r_{1,m})\Big)\Big)\,(1+\Upsilon_{k,m})-$$

$$3\,\beta_0^2\,\hat{\beta}_a\,\Big(2\,d_{11}+d_{22}\,\Big(-2+\hat{\beta}_a-12\,r_{1,m}\Big)\Big)\,(1+\Upsilon_{k,m})^2+6\,d_{22}\,\beta_0^3\,\hat{\beta}_a^2\,r_{1,m}\,(1+\Upsilon_{k,m})^3\Big)\Big)+$$

$$\hat{\chi}\,d_{11}\,\alpha_2\,\hat{\beta}_a\,\Big(d_{11}\,\beta_0\,(1+\Upsilon_{k,m})\,\Big(-17+\beta_0\,\hat{\beta}_a\,(1+\Upsilon_{k,m})\Big)-$$

$$d_{22}\,(-3+\beta_0\,(4+(4+6\,r_{1,m})\,\Upsilon_{k,m}))\Big)+d_{22}\,\alpha_3^2\,\Big(-2\,d_{11}\,d_{22}\,(3\,q_1+q_2)\,\hat{\beta}_a\,(1+2\,\beta_0\,r_{1,m})+$$

$$\beta_0\,\Big(4\,d_{11}^2\,(3\,q_1+4\,q_2)\,\hat{\beta}_a+12\,d_0\,d_{22}\,\hat{\beta}_a^2\,r_{1,m}+d_{11}\,d_{22}\,\Big(2\,(3\,q_1+q_2)\,\hat{\beta}_a\,(1+2\,r_{1,m})+$$

$$6\,\hat{\chi}\,d_{22}\,\alpha_2\,(1+\beta_0\,r_{1,m})+\hat{\beta}_a^2\,(2\,q_2\,(1+\beta_0\,r_{1,m})+q_1\,(-3+6\,\beta_0\,r_{1,m}))\Big)\Big)$$

$$(1+\Upsilon_{k,m})+d_{11}\,\beta_0^2\,\Big(\hat{\chi}\,d_{22}\,\alpha_2\,\Big(-20\,d_{11}+d_{22}\,\Big(2+3\,\hat{\beta}_a-6\,r_{1,m}\Big)\Big)+$$

$$\hat{\beta}_a^2\,(6\,d_{11}\,(2\,q_1-q_2)-d_{22}\,(3\,q_1+q_2)\,(1+2\,r_{1,m}))\Big)\,(1+\Upsilon_{k,m})^2+$$

$$\hat{\chi}\,d_{11}\,d_{22}\,(-20\,d_{11}+d_{22})\,\alpha_2\,\beta_0^3\,\hat{\beta}_a\,(1+\Upsilon_{k,m})^3+6\,d_0\,\hat{\beta}_a^2\,(1+\epsilon_{s,m})$$

$$(d_{11}\,\beta_0\,(1+\Upsilon_{k,m})-d_{22}\,(-1+\beta_0\,(1+\Upsilon_{k,m}+r_{1,m}\,(2+4\,\Upsilon_{k,m}))))\Big)\Big)+\alpha_1$$

$$\Big(-\hat{\chi}\,d_{11}\,d_{22}\,\alpha_2\,\alpha_3\,\hat{\beta}_a\,\Big(-4\,d_{22}\,(1+2\,\beta_0\,r_{1,m})-2\,\beta_0\,\Big(-3\,d_{11}+d_{22}\,\Big(-3-4\,r_{1,m}+\hat{\beta}_a\,(1+\beta_0\,r_{1,m})\Big)\Big)$$

$$(1+\Upsilon_{k,m})+\beta_0^2\,\hat{\beta}_a\,(16\,d_{11}+d_{22}\,(1+2\,r_{1,m}))\,(1+\Upsilon_{k,m})^2\Big)+$$

$$d_{11}\,d_{22}\,\alpha_3^2\,\Big(d_{22}\,\Big(\hat{\chi}\,d_{22}\,\alpha_2-(3\,q_1+q_2)\,\hat{\beta}_a^2\Big)\,(1+2\,\beta_0\,r_{1,m})+$$

$$\beta_0\,\Big(\hat{\beta}_a^2\,(d_{11}\,(6\,q_1+8\,q_2)+d_{22}\,(3\,q_1+q_2)\,(1+2\,r_{1,m}))+$$

$$\hat{\chi}\,d_{22}\,\alpha_2\,\Big(-3\,d_{11}+2\,d_{22}\,\Big(-r_{1,m}+4\,\hat{\beta}_a\,(1+\beta_0\,r_{1,m})\Big)\Big)\Big)\,(1+\Upsilon_{k,m})+\hat{\chi}\,d_{22}\,\alpha_2\,\beta_0^2\,\hat{\beta}_a$$

$$\Big(-17\,d_{11}+d_{22}\,\Big(-7+\hat{\beta}_a-8\,r_{1,m}\Big)\Big)\,(1+\Upsilon_{k,m})^2-8\,\hat{\chi}\,d_{11}\,d_{22}\,\alpha_2\,\beta_0^3\,\hat{\beta}_a^2\,(1+\Upsilon_{k,m})^3\Big)-$$

$$4\,d_0\,d_{22}^6\,\alpha_3^6\,\beta_0^2\,\hat{\beta}_a\,(1+\Upsilon_{k,m})^2\,(-1+\epsilon_{s,m}\,(-1+2\,\beta_0\,r_{1,m}\,(1+\Upsilon_{k,m})))+$$

$$2\,d_0\,d_{22}^4\,\alpha_3^5\,\beta_0\,\hat{\beta}_a\,(1+\Upsilon_{k,m})$$

$$\Big(2\,d_{22}\,\beta_0\,r_{1,m}\,(1+\Upsilon_{k,m})\,\Big(4+3\,\beta_0\,\hat{\beta}_a\,(1+\Upsilon_{k,m})\Big)+(1+\epsilon_{s,m})\,\Big(4\,d_{22}\,(1+\beta_0\,r_{1,m})+$$

$$\beta_0\,\Big(2\,d_{11}+d_{22}\,\Big(-2+3\,\hat{\beta}_a-12\,r_{1,m}\Big)\Big)\,(1+\Upsilon_{k,m})-6\,d_{22}\,\beta_0^2\,\hat{\beta}_a\,r_{1,m}\,(1+\Upsilon_{k,m})^2\Big)\Big)+$$

$$d_{22}^3\,\alpha_3^4\,\Big(\beta_0\,(1+\Upsilon_{k,m})\,\Big(2\,d_{22}\,\hat{\beta}_a\,(4\,d_0\,r_{1,m}+d_{11}\,(q_1+q_2)\,(-1+2\,\beta_0\,r_{1,m}))+$$

$$\beta_0\,\Big(8\,d_{11}^2\,(q_1+q_2)\,\hat{\beta}_a+24\,d_0\,d_{22}\,\hat{\beta}_a^2\,r_{1,m}+$$

$$d_{11}\,d_{22}\,\Big(\hat{\chi}\,d_{22}\,\alpha_2+q_2\,\hat{\beta}_a^2-2\,(q_1+q_2)\,\hat{\beta}_a\,(1+2\,r_{1,m})\Big)\Big)\,(1+\Upsilon_{k,m})+$$

$$d_{11}\,\beta_0^2\,\Big(\hat{\chi}\,d_{22}\,(-4\,d_{11}+d_{22})\,\alpha_2+2\,d_{11}\,q_2\,\hat{\beta}_a^2\Big)\,(1+\Upsilon_{k,m})^2\Big)+2\,d_0\,\hat{\beta}_a\,(1+\epsilon_{s,m})$$

$$\Big(2\,d_{22}\,(1+2\,\beta_0\,r_{1,m})+2\,\beta_0\,\Big(d_{11}+d_{22}\,\Big(-1-4\,r_{1,m}+3\,\hat{\beta}_a\,(1+\beta_0\,r_{1,m})\Big)\Big)\,(1+\Upsilon_{k,m})+$$

$$3\,\beta_0^2\,\hat{\beta}_a\,(d_{11}-d_{22}\,(1+6\,r_{1,m}))\,(1+\Upsilon_{k,m})^2\Big)\Big)+$$

$$\hat{\chi}\,d_{11}\,\alpha_2\,\hat{\beta}_a^2\,(-8\,d_{11}\,\beta_0\,(1+\Upsilon_{k,m})-d_{22}\,(-1+\beta_0\,(1+(1+2\,r_{1,m})\,\Upsilon_{k,m})))+$$

$$d_{22}^2\,\alpha_3^3\,\Big(-2\,d_{11}\,d_{22}\,(q_1+q_2)\,\hat{\beta}_a\,(1+2\,\beta_0\,r_{1,m})+$$

$$\beta_0\,\Big(4\,d_{11}^2\,(q_1+q_2)\,\hat{\beta}_a+12\,d_0\,d_{22}\,\hat{\beta}_a^2\,r_{1,m}+d_{11}\,d_{22}\,\Big(2\,(q_1+q_2)\,\hat{\beta}_a\,(1+2\,r_{1,m})+$$

$$2\,\hat{\chi}\,d_{22}\,\alpha_2\,(1+\beta_0\,r_{1,m})+\hat{\beta}_a^2\,(6\,q_2\,\beta_0\,r_{1,m}+q_1\,(-3+6\,\beta_0\,r_{1,m}))\Big)\Big)$$
$$(1+\Upsilon_{k,m})+d_{11}\,\beta_0^2\,\Big(\hat{\chi}\,d_{22}\,\alpha_2\,\big(-7\,d_{11}+d_{22}\,\big(1+4\,\hat{\beta}_a-2\,r_{1,m}\big)\big)+$$
$$\hat{\beta}_a^2\,(2\,d_{11}\,(6\,q_1+7\,q_2)-3\,d_{22}\,(q_1+q_2)\,(1+2\,r_{1,m}))\Big)\,(1+\Upsilon_{k,m})^2-$$
$$\hat{\chi}\,d_{11}\,d_{22}\,(11\,d_{11}+d_{22})\,\alpha_2\,\beta_0^3\,\hat{\beta}_a\,(1+\Upsilon_{k,m})^3+6\,d_0\,\hat{\beta}_a^2\,(1+\epsilon_{s,m})$$
$$(d_{11}\,\beta_0\,(1+\Upsilon_{k,m})-d_{22}\,(-1+\beta_0\,(1+\Upsilon_{k,m}+r_{1,m}\,(2+4\,\Upsilon_{k,m}))))\Big)\Big)\Big)$$

---

$$p_{8\,(4)}=\frac{1}{8\,d_{22}^2\,\alpha_3\,(1+d_{22}\,\alpha_3\,\beta_0\,(1+\Upsilon_{k,m}))^3}\,d_{11}\,\beta_0\,(1+\Upsilon_{k,m})$$
$$\Big(d_{22}\,q_1\,\big(-4\,d_{22}^2\,\alpha_3\,\beta_0\,(1+(1+2\,r_{1,m})\,\Upsilon_{k,m})+d_{11}\,(-1+d_{22}\,\alpha_3\,\beta_0\,(1+\Upsilon_{k,m}))\big)+$$
$$\frac{1}{(\alpha_1+\alpha_3)^2}d_{22}\,q_2\,(\alpha_1-\alpha_3)\,\big(4\,d_{22}^2\,(\alpha_1+\alpha_3)^2\,\beta_0\,(1+(1+2\,r_{1,m})\,\Upsilon_{k,m})+$$
$$d_{11}\,\big(-\alpha_3\,(-1+d_{22}\,\alpha_3\,\beta_0\,(1+\Upsilon_{k,m}))+d_{22}\,\alpha_1^2\,\beta_0\,(1+\Upsilon_{k,m})\,(-1+d_{22}\,\alpha_3\,\beta_0\,(1+\Upsilon_{k,m}))+$$
$$\alpha_1\,\big(7+10\,d_{22}\,\alpha_3\,\beta_0\,(1+\Upsilon_{k,m})+7\,d_{22}^2\,\alpha_3^2\,\beta_0^2\,(1+\Upsilon_{k,m})^2\big)\big)\big)+$$
$$1\Big/\Big(\alpha_1\,(\alpha_1+\alpha_3)^3\,\big(d_{22}\,\alpha_1+\hat{\beta}_a\big)^2\Big)\,(1+d_{22}\,\alpha_3\,\beta_0\,(1+\Upsilon_{k,m}))\,\Big(-4\,d_0\,d_{22}^4\,\alpha_1^6\,\alpha_3\,(1+\epsilon_{s,m})-$$
$$4\,d_{22}^3\,\alpha_1^5\,\big(d_0\,\alpha_3\,\big(3\,d_{22}\,\alpha_3+2\,\hat{\beta}_a\big)\,(1+\epsilon_{s,m})-\hat{\chi}\,d_{22}\,\alpha_2\,\beta_0\,(1+\Upsilon_{k,m})\big)+$$
$$\hat{\chi}\,d_{11}\,\alpha_2\,\alpha_3^2\,\hat{\beta}_a\,\big(d_{22}\,\alpha_3+\hat{\beta}_a\big)\,(1+d_{22}\,\alpha_3\,\beta_0\,(1+\Upsilon_{k,m}))+$$
$$4\,d_{22}^2\,\alpha_1^4\,\Big(-3\,d_0\,d_{22}^2\,\alpha_3^3\,(1+\epsilon_{s,m})-6\,d_0\,d_{22}\,\alpha_3^2\,\hat{\beta}_a\,(1+\epsilon_{s,m})+\alpha_3\,\Big(-d_0\,\hat{\beta}_a^2\,(1+\epsilon_{s,m})+$$
$$\hat{\chi}\,d_{22}\,(d_{11}+3\,d_{22})\,\alpha_2\,\beta_0\,(1+\Upsilon_{k,m})\Big)+\hat{\chi}\,(d_{11}+d_{22})\,\alpha_2\,\big(1+\beta_0\,\hat{\beta}_a\,(1+\Upsilon_{k,m})\big)\Big)+$$
$$\alpha_1\,\alpha_3\,\Big(3\,\hat{\chi}\,d_{11}\,\alpha_2\,\hat{\beta}_a^2-d_{22}^2\,\alpha_3^3\,\Big(4\,d_0\,\hat{\beta}_a^2\,(1+\epsilon_{s,m})+\hat{\chi}\,(d_{11}-4\,d_{22})\,d_{22}\,\alpha_2\,\beta_0\,(1+\Upsilon_{k,m})\Big)+$$
$$\hat{\chi}\,d_{22}\,\alpha_2\,\alpha_3\,\hat{\beta}_a\,\big(4\,d_{22}+5\,d_{11}\,\beta_0\,\hat{\beta}_a\,(1+\Upsilon_{k,m})\big)+$$
$$\hat{\chi}\,d_{22}^2\,\alpha_2\,\alpha_3^2\,\big(4\,d_{22}\,\big(1+\beta_0\,\hat{\beta}_a\,(1+\Upsilon_{k,m})\big)+d_{11}\,\big(-1+2\,\beta_0\,\hat{\beta}_a\,(1+\Upsilon_{k,m})\big)\big)\Big)-$$
$$2\,d_{22}\,\alpha_1^3\,\Big(2\,d_0\,d_{22}^3\,\alpha_3^4\,(1+\epsilon_{s,m})+12\,d_0\,d_{22}^2\,\alpha_3^3\,\hat{\beta}_a\,(1+\epsilon_{s,m})+2\,d_{22}\,\alpha_3^2\,\Big(3\,d_0\,\hat{\beta}_a^2\,(1+\epsilon_{s,m})+$$
$$\hat{\chi}\,(d_{11}-4\,d_{22})\,d_{22}\,\alpha_2\,\beta_0\,(1+\Upsilon_{k,m})\Big)-2\,\hat{\chi}\,\alpha_2\,\hat{\beta}_a\,\big(d_{22}+d_{11}\,\big(3+\beta_0\,\hat{\beta}_a\,(1+\Upsilon_{k,m})\big)\big)-$$
$$3\,\hat{\chi}\,d_{22}\,\alpha_2\,\alpha_3\,\big(2\,d_{22}\,\big(1+\beta_0\,\hat{\beta}_a\,(1+\Upsilon_{k,m})\big)+d_{11}\,\big(-1+3\,\beta_0\,\hat{\beta}_a\,(1+\Upsilon_{k,m})\big)\big)\Big)+$$
$$\alpha_1^2\,\Big(8\,\hat{\chi}\,d_{11}\,\alpha_2\,\hat{\beta}_a^2-8\,d_0\,d_{22}^3\,\alpha_3^4\,\hat{\beta}_a\,(1+\epsilon_{s,m})-3\,d_{22}^2\,\alpha_3^3$$
$$\Big(4\,d_0\,\hat{\beta}_a^2\,(1+\epsilon_{s,m})+\hat{\chi}\,(d_{11}-4\,d_{22})\,d_{22}\,\alpha_2\,\beta_0\,(1+\Upsilon_{k,m})\Big)+$$
$$\hat{\chi}\,d_{22}^2\,\alpha_2\,\alpha_3^2\,\big(12\,d_{22}\,\big(1+\beta_0\,\hat{\beta}_a\,(1+\Upsilon_{k,m})\big)+d_{11}\,\big(-5+3\,\beta_0\,\hat{\beta}_a\,(1+\Upsilon_{k,m})\big)\big)+$$
$$\hat{\chi}\,d_{22}\,\alpha_2\,\alpha_3\,\hat{\beta}_a\,\big(8\,d_{22}+d_{11}\,\big(-1+14\,\beta_0\,\hat{\beta}_a\,(1+\Upsilon_{k,m})\big)\big)\Big)\Big)\Big)$$

---

$$
\begin{aligned}
p_{9\,(4)} = {} & \frac{1}{4\, d_{22}^{2}\, \alpha_3\, (1 + d_{22}\, \alpha_3\, \beta_0\, (1 + \Upsilon_{k,m}))^{3}}\, \beta_0\, (1 + \Upsilon_{k,m}) \\
& (-d_{11}\, d_{22}\, q_1\, (d_{12} + 3\, d_{12}\, d_{22}\, \alpha_3\, \beta_0\, (1 + \Upsilon_{k,m}) + d_{21}\, d_{22}\, \alpha_3\, \beta_0\, (1 + \Upsilon_{k,m})\, (2 - d_{22}\, \alpha_3\, \beta_0\, (1 + \Upsilon_{k,m}))) + \\
& d_{11}\, d_{22}\, q_2\, (-d_{12}\, (1 + 3\, d_{22}\, \alpha_3\, \beta_0\, (1 + \Upsilon_{k,m}) + d_{22}\, \alpha_1\, \beta_0\, (1 + \Upsilon_{k,m})\, (-1 + d_{22}\, \alpha_3\, \beta_0\, (1 + \Upsilon_{k,m}))) + \\
& d_{21}\, d_{22}\, \beta_0\, (1 + \Upsilon_{k,m})\, (\alpha_3\, (-2 + d_{22}\, \alpha_3\, \beta_0\, (1 + \Upsilon_{k,m})) + \alpha_1\, (2 + d_{22}^{2}\, \alpha_3^{2}\, \beta_0^{2}\, (1 + \Upsilon_{k,m})^{2}))) + \\
& 1 \Big/ (\alpha_1\, (\alpha_1 - \alpha_3)^{2}\, (\alpha_1 + \alpha_3)^{2}\, (d_{22}\, \alpha_1 + \hat{\beta}_a)^{2})\, (1 + d_{22}\, \alpha_3\, \beta_0\, (1 + \Upsilon_{k,m})) \\
& (2\, d_0\, (d_{12} - d_{21})\, d_{22}^{4}\, \alpha_1^{7}\, \alpha_3\, (1 + \epsilon_{s,m}) + 4\, d_0\, (d_{12} - d_{21})\, d_{22}^{3}\, \alpha_1^{6}\, \alpha_3\, \hat{\beta}_a\, (1 + \epsilon_{s,m}) + 2\, d_{22}^{2}\, \alpha_1^{5} \\
& (\hat{\chi}\, d_{11}\, (d_{12} + d_{21})\, \alpha_2 + 2\, d_0\, (-d_{12} + d_{21})\, d_{22}^{2}\, \alpha_3^{3}\, (1 + \epsilon_{s,m}) + d_0\, (d_{12} - d_{21})\, \alpha_3\, \hat{\beta}_a^{2}\, (1 + \epsilon_{s,m})) + \\
& \hat{\chi}\, d_{11}\, (d_{12} + d_{21})\, \alpha_2\, \alpha_3^{3}\, \hat{\beta}_a\, (d_{22}\, \alpha_3 + \hat{\beta}_a)\, (1 + d_{22}\, \alpha_3\, \beta_0\, (1 + \Upsilon_{k,m})) + 2\, d_{22}\, \alpha_1^{4} \\
& (\hat{\chi}\, d_{11}\, (d_{12} + 4\, d_{21})\, d_{22}\, \alpha_2\, \alpha_3 + 2\, \hat{\chi}\, d_{11}\, (d_{12} + d_{21})\, \alpha_2\, \hat{\beta}_a + \hat{\chi}\, d_{11}\, (2\, d_{12} + 5\, d_{21})\, d_{22}^{2}\, \alpha_2\, \alpha_3^{2}\, \beta_0 \\
& (1 + \Upsilon_{k,m}) + 2\, d_{22}^{2}\, \alpha_3^{3}\, (2\, d_0\, (-d_{12} + d_{21})\, \hat{\beta}_a\, (1 + \epsilon_{s,m}) + \hat{\chi}\, d_{11}\, d_{21}\, d_{22}\, \alpha_2\, \beta_0^{2}\, (1 + \Upsilon_{k,m})^{2})) + \\
& d_{22}\, \alpha_1\, \alpha_3^{3}\, (3\, \hat{\chi}\, d_{11}\, (d_{12} + d_{21})\, \alpha_2\, \hat{\beta}_a + d_{22}\, \alpha_3^{2}\, (2\, d_0\, (d_{12} - d_{21})\, \hat{\beta}_a^{2}\, (1 + \epsilon_{s,m}) + \\
& \hat{\chi}\, d_{11}\, (3\, d_{12} + 5\, d_{21})\, d_{22}\, \alpha_2\, \beta_0\, (1 + \Upsilon_{k,m})) + \\
& \hat{\chi}\, d_{11}\, d_{22}\, \alpha_2\, \alpha_3\, (3\, d_{12}\, (1 + \beta_0\, \hat{\beta}_a\, (1 + \Upsilon_{k,m})) + d_{21}\, (5 + 3\, \beta_0\, \hat{\beta}_a\, (1 + \Upsilon_{k,m})))) + \\
& \alpha_1^{2}\, \alpha_3\, (\hat{\chi}\, d_{11}\, (-3\, d_{12} + d_{21})\, \alpha_2\, \hat{\beta}_a^{2} + 4\, d_0\, (d_{12} - d_{21})\, d_{22}^{3}\, \alpha_3^{4}\, \hat{\beta}_a\, (1 + \epsilon_{s,m}) - \\
& 2\, \hat{\chi}\, d_{11}\, d_{21}\, d_{22}^{3}\, \alpha_2\, \alpha_3^{3}\, \beta_0\, (1 + \Upsilon_{k,m}) - \\
& \hat{\chi}\, d_{11}\, d_{22}\, \alpha_2\, \alpha_3\, \hat{\beta}_a\, (d_{21}\, (5 - 3\, \beta_0\, \hat{\beta}_a\, (1 + \Upsilon_{k,m})) + d_{12}\, (5 + \beta_0\, \hat{\beta}_a\, (1 + \Upsilon_{k,m}))) + \hat{\chi}\, d_{11}\, d_{22}^{2} \\
& \alpha_2\, \alpha_3^{2}\, (-5\, d_{12}\, \beta_0\, \hat{\beta}_a\, (1 + \Upsilon_{k,m}) + d_{21}\, (-2 - 5\, \beta_0\, \hat{\beta}_a\, (1 + \Upsilon_{k,m}) + 4\, \beta_0^{2}\, \hat{\beta}_a^{2}\, (1 + \Upsilon_{k,m})^{2}))) + \\
& \alpha_1^{3}\, (\hat{\chi}\, d_{11}\, (-3\, d_{12} + 5\, d_{21})\, d_{22}\, \alpha_2\, \alpha_3\, \hat{\beta}_a + 2\, \hat{\chi}\, d_{11}\, (d_{12} + d_{21})\, \alpha_2\, \hat{\beta}_a^{2} + \\
& 2\, d_0\, (d_{12} - d_{21})\, d_{22}^{4}\, \alpha_3^{5}\, (1 + \epsilon_{s,m}) + \hat{\chi}\, d_{11}\, d_{22}^{2}\, \alpha_2\, \alpha_3^{2}\, (d_{12}\, (-7 + \beta_0\, \hat{\beta}_a\, (1 + \Upsilon_{k,m})) + \\
& 9\, d_{21}\, (-1 + \beta_0\, \hat{\beta}_a\, (1 + \Upsilon_{k,m}))) + d_{22}^{2}\, \alpha_3^{3}\, (4\, d_0\, (-d_{12} + d_{21})\, \hat{\beta}_a^{2}\, (1 + \epsilon_{s,m}) + \\
& \hat{\chi}\, d_{11}\, d_{22}\, \alpha_2\, \beta_0\, (1 + \Upsilon_{k,m})\, (-7\, d_{12} + d_{21}\, (-9 + 8\, \beta_0\, \hat{\beta}_a\, (1 + \Upsilon_{k,m}))))))))
\end{aligned}
$$

$$p_{10\,(4)} = \frac{1}{2\,(1 + d_{22}\,\alpha_3\,\beta_0\,(1 + \Upsilon_{k,m}))^3}\,d_{11}\,\beta_0\,(1 + \Upsilon_{k,m})$$
$$\Bigg(q_1\,\beta_0\,(d_{11}\,(1 + \Upsilon_{k,m}) - d_{22}\,(1 + (1 + 2\,r_{1,m})\,\Upsilon_{k,m})) + \frac{1}{d_{22}\,\alpha_3\,(\alpha_1 + \alpha_3)^2}$$
$$q_2\,(\alpha_1 - \alpha_3)\,\Big(d_{22}^2\,(\alpha_1 + \alpha_3)^2\,\beta_0\,(1 + (1 + 2\,r_{1,m})\,\Upsilon_{k,m}) + d_{11}\,\Big(-d_{22}\,\alpha_3^2\,\beta_0\,(1 + \Upsilon_{k,m}) +$$
$$d_{22}^2\,\alpha_1^2\,\alpha_3\,\beta_0^2\,(1 + \Upsilon_{k,m})^2 + \alpha_1\,\Big(2 + 3\,d_{22}\,\alpha_3\,\beta_0\,(1 + \Upsilon_{k,m}) + 3\,d_{22}^2\,\alpha_3^2\,\beta_0^2\,(1 + \Upsilon_{k,m})^2\Big)\Big)\Big) +$$
$$1\Big/\Big(d_{22}^2\,\alpha_3\,(\alpha_1 + \alpha_3)^3\,\big(d_{22}\,\alpha_1 + \hat{\beta}_a\big)^2\Big)\,\hat{\chi}\,\alpha_2\,(1 + d_{22}\,\alpha_3\,\beta_0\,(1 + \Upsilon_{k,m}))$$
$$\Big(d_{22}^4\,\alpha_1^4\,\beta_0\,(1 + \Upsilon_{k,m}) - (d_{11} - d_{22})\,d_{22}\,\alpha_3^2\,\big(d_{22}\,\alpha_3 + \hat{\beta}_a\big)\,(1 + d_{22}\,\alpha_3\,\beta_0\,(1 + \Upsilon_{k,m})) +$$
$$d_{22}^2\,\alpha_1^3\,\Big(d_{11} + d_{11}\,\beta_0\,\hat{\beta}_a\,(1 + \Upsilon_{k,m}) + d_{22}\,\Big(1 + 3\,d_{22}\,\alpha_3\,\beta_0\,(1 + \Upsilon_{k,m}) + \beta_0\,\hat{\beta}_a\,(1 + \Upsilon_{k,m})\Big)\Big) +$$
$$d_{22}\,\alpha_1^2\,\Big(4\,d_{22}^2\,(-d_{11} + d_{22})\,\alpha_3^2\,\beta_0\,(1 + \Upsilon_{k,m}) + 3\,d_{22}\,\alpha_3\,\Big(d_{11}\,\Big(-1 + \beta_0\,\hat{\beta}_a\,(1 + \Upsilon_{k,m})\Big) +$$
$$d_{22}\,\Big(1 + \beta_0\,\hat{\beta}_a\,(1 + \Upsilon_{k,m})\Big)\Big) + \hat{\beta}_a\,\Big(d_{22} + d_{11}\,\Big(3 + \beta_0\,\hat{\beta}_a\,(1 + \Upsilon_{k,m})\Big)\Big)\Big) +$$
$$\alpha_1\,\Big(2\,d_{11}\,\hat{\beta}_a^2 + 3\,d_{22}^3\,(-d_{11} + d_{22})\,\alpha_3^3\,\beta_0\,(1 + \Upsilon_{k,m}) - 3\,(d_{11} - d_{22})\,d_{22}^2\,\alpha_3^2$$
$$\Big(1 + \beta_0\,\hat{\beta}_a\,(1 + \Upsilon_{k,m})\Big) + d_{22}\,\alpha_3\,\hat{\beta}_a\,\Big(2\,d_{22} + d_{11}\,\Big(-2 + 3\,\beta_0\,\hat{\beta}_a\,(1 + \Upsilon_{k,m})\Big)\Big)\Big)\Big)\Bigg)$$

---

$$p_{11\,(4)} = \frac{1}{8\,d_{22}^2\,\alpha_3^2\,(1 + d_{22}\,\alpha_3\,\beta_0\,(1 + \Upsilon_{k,m}))^3}\,d_{11}\,\beta_0\,(1 + \Upsilon_{k,m})$$
$$\Bigg(-d_{11}\,d_{22}\,q_1\,(1 + 3\,d_{22}\,\alpha_3\,\beta_0\,(1 + \Upsilon_{k,m})) - \frac{1}{(\alpha_1 + \alpha_3)^2}\,d_{11}\,d_{22}\,q_2\,(\alpha_1 - \alpha_3)$$
$$\Big(-\alpha_3\,(1 + 3\,d_{22}\,\alpha_3\,\beta_0\,(1 + \Upsilon_{k,m})) + d_{22}\,\alpha_1^2\,\beta_0\,(1 + \Upsilon_{k,m})\,(1 + 3\,d_{22}\,\alpha_3\,\beta_0\,(1 + \Upsilon_{k,m})) +$$
$$\alpha_1\,\Big(1 + 2\,d_{22}\,\alpha_3\,\beta_0\,(1 + \Upsilon_{k,m}) + 5\,d_{22}^2\,\alpha_3^2\,\beta_0^2\,(1 + \Upsilon_{k,m})^2\Big)\Big) + 1\Big/\Big(\alpha_1^2\,(\alpha_1 + \alpha_3)^3\,\big(d_{22}\,\alpha_1 + \hat{\beta}_a\big)^2\Big)$$
$$\alpha_3\,(1 + d_{22}\,\alpha_3\,\beta_0\,(1 + \Upsilon_{k,m}))\,\Big(-4\,d_0\,d_{22}^4\,\alpha_1^7\,(1 + \epsilon_{s,m}) - 4\,d_0\,d_{22}^3\,\alpha_1^6\,\big(3\,d_{22}\,\alpha_3 + 2\,\hat{\beta}_a\big)\,(1 + \epsilon_{s,m}) -$$
$$4\,d_{22}^2\,\alpha_1^5\,\Big(d_0\,\Big(3\,d_{22}^2\,\alpha_3^2 + 6\,d_{22}\,\alpha_3\,\hat{\beta}_a + \hat{\beta}_a^2\Big)\,(1 + \epsilon_{s,m}) - \hat{\chi}\,d_{11}\,d_{22}\,\alpha_2\,\beta_0\,(1 + \Upsilon_{k,m})\Big) +$$
$$\hat{\chi}\,d_{11}\,\alpha_2\,\alpha_3^2\,\hat{\beta}_a\,\big(d_{22}\,\alpha_3 + \hat{\beta}_a\big)\,(1 + d_{22}\,\alpha_3\,\beta_0\,(1 + \Upsilon_{k,m})) + 3\,\hat{\chi}\,d_{11}\,\alpha_1\,\alpha_2\,\alpha_3\,\big(d_{22}\,\alpha_3 + \hat{\beta}_a\big)^2$$
$$(1 + d_{22}\,\alpha_3\,\beta_0\,(1 + \Upsilon_{k,m})) - 2\,d_{22}^2\,\alpha_1^4\,\Big(2\,d_0\,\alpha_3\,\Big(d_{22}^2\,\alpha_3^2 + 6\,d_{22}\,\alpha_3\,\hat{\beta}_a + 3\,\hat{\beta}_a^2\Big)\,(1 + \epsilon_{s,m}) -$$
$$3\,\hat{\chi}\,d_{11}\,\alpha_2\,\Big(1 + 2\,d_{22}\,\alpha_3\,\beta_0\,(1 + \Upsilon_{k,m}) + \beta_0\,\hat{\beta}_a\,(1 + \Upsilon_{k,m})\Big)\Big) -$$
$$2\,d_{22}\,\alpha_1^3\,\Big(2\,d_0\,d_{22}\,\alpha_3^2\,\hat{\beta}_a\,\big(2\,d_{22}\,\alpha_3 + 3\,\hat{\beta}_a\big)\,(1 + \epsilon_{s,m}) - \hat{\chi}\,d_{11}\,\alpha_2$$
$$\Big(6\,d_{22}^2\,\alpha_3^2\,\beta_0\,(1 + \Upsilon_{k,m}) + \hat{\beta}_a\,\Big(5 + \beta_0\,\hat{\beta}_a\,(1 + \Upsilon_{k,m})\Big) + d_{22}\,\alpha_3\,\Big(5 + 9\,\beta_0\,\hat{\beta}_a\,(1 + \Upsilon_{k,m})\Big)\Big)\Big) +$$
$$\alpha_1^2\,\Big(-4\,d_0\,d_{22}^2\,\alpha_3^3\,\hat{\beta}_a^2\,(1 + \epsilon_{s,m}) + \hat{\chi}\,d_{11}\,\alpha_2\,\Big(4\,\hat{\beta}_a^2 + 9\,d_{22}^3\,\alpha_3^3\,\beta_0\,(1 + \Upsilon_{k,m}) +$$
$$d_{22}\,\alpha_3\,\hat{\beta}_a\,\Big(11 + 6\,\beta_0\,\hat{\beta}_a\,(1 + \Upsilon_{k,m})\Big) + d_{22}^2\,\alpha_3^2\,\Big(9 + 13\,\beta_0\,\hat{\beta}_a\,(1 + \Upsilon_{k,m})\Big)\Big)\Big)\Big)\Bigg)$$

---
